# Supplementary material for: CAD-Deform: Deformable Fitting of CAD Models to 3D Scans
Source: arXiv:2007.11965 source file (2020-07-23)
Supplement: Supplementary file 1 [file suppl_B_deformation_details.tex]

\newcommand{\bE}{\mathbf{E}}
\newcommand{\bV}{\mathbf{V}}

\newcommand{\bd}{\mathbf{d}}
\newcommand{\bp}{\mathbf{p}}

\section{Deformation Algorithm Details}

Here we are going to provide readers with the details of mesh deformation framework implementation. In energy equation~\ref{} consider term $E_0 = \sum_{e \in \bE}\|T_e(\bV) - T_e^0\|^2_2$, where $T_e$ is $4 \times 4$ affine transformation matrix having $[0, 0, 0, 1]$ in the last row. Transformation $T_e$ can be considered as a pair $(C, \bd)$, where $C$ is $3 \times 3$ and $\bd$ is a vector of size $3$, so that the transform is $\bp = C\bp_0 + \bd$.
