# Supplementary material for: CAD-Deform: Deformable Fitting of CAD Models to 3D Scans
Source: arXiv:2007.11965 source file (2020-07-23)
Supplement: Supplementary file 2 [file suppl_D_dame.tex]

\section{More detailed results on local surface quality evaluation}
\label{supsec:more_dame}
